# Supplementary material for: ezDPS: An Efficient and Zero-Knowledge Machine Learning Inference Pipeline
Source: arXiv:2212.05428 source file (2023-02-01)
Supplement: Supplementary file 1 [file appendix.tex]

\section*{A. Algorithms for Machine Learning Operators}
\begin{algorithm}
	\caption{Daubechies DB4 decomposition}
	\label{db decom}
	\begin{algorithmic}[1]
		\REQUIRE
		data=[$a_0$, $a_1$, ..., $a_{n-1}$]
		\ENSURE
		The wavelet decomposition result: out = [$o_0, o_1, ..., o_{n-1}$]
		\STATE n = len(data)
		\IF{$n<4$}
		\STATE raise valuewerror
		\ELSE
		\STATE half = $n >> 1$
		\STATE i = 0
		\FOR{$j = 0$; $j < n - 3$; $j = j + 2$}
		\STATE out[i] = data[j] $\times$ h0 + data[j+1] $\times h_1$ + data[j+2] $\times h_2$ + data[j+3] $\times h_3$
		\STATE out[i+half] = data[j] $\times g_0$ + data[j+1] $\times g_1$ + data[j+2] $\times g_2$ + data[j+3] $\times g_3$
		\STATE i = i + 1
		\ENDFOR
		\STATE out[i] = data[n - 2] $\times h_0$ + data[n - 1] $\times h_1$ + data[0] $\times h_2$ + data[1] $\times h_3$
		\STATE out[i + half] = data[n - 2] $\times g_0$ + data[n - 1] $\times g_1$ + data[0] $\times g_2$ + data[1] $\times g_3$
		\ENDIF
	\end{algorithmic}
\end{algorithm}

\begin{algorithm}
	\caption{Wavelet thresholding function}
	\label{db thre}
	\begin{algorithmic}[1]
		\REQUIRE
		data = [$a_0$, $a_1$, ..., $a_{n-1}$], threshold $thr$
		\ENSURE
		The data after thresholding: out =  [$o_0, o_1, ..., o_{n-1}$]
		\STATE n = len(data)
		\FOR{$i = 0$; $i < n$; $i ++$}
		\STATE // abs($\cdot$) is a function used to compute the absolute value
		\STATE temp = data[i] / abs(data[i]) 
		\STATE comp = temp - thr
		\IF{comp $> 0$}
		\STATE out[i] = temp $\times$ comp
		\ELSE
		\STATE out[i] = 0
		\ENDIF
		\ENDFOR
	\end{algorithmic}
\end{algorithm}

\begin{algorithm}
	\caption{Daubechies DB4 reconstruction}
	\label{db rec}
	\begin{algorithmic}[1]
		\REQUIRE
		data = [$a_0$, $a_1$, ..., $a_{n-1}$]
		\ENSURE
		The reconstruct data of : out =  [$o_0, o_1, ..., o_{n-1}$]
		\STATE n = len(data)
		\IF{$n<4$}
		\STATE raise valuewerror
		\ELSE
		\STATE half = $n >> 1$
		\STATE half\_plus = half + 1
		\STATE out[0] = data[half-1] $\times Ih_0$ + data[n-1] $\times Ih_1$ + data[0] $\times Ih_2$ + data[half] $\times Ih_3$
		\STATE out[1] = data[half - 1] $\times Ig_0$ + data[n - 1] $\times Ig_1$ + data[0] $\times Ig_2$ + data[half] $\times Ig_3$
		\STATE j = 2
		\FOR{$i = 0$; $i < half - 1$; $i = i + 1$}
		\STATE temp[j ++] = data[i] $\times Ih_0$ + data[i + half] $\times Ih_1$ + data[i + 1] $\times Ih_2$ + data[i + halfplus] $\times Ih_3$
		\STATE temp[j ++] = data[i] $\times Ig_0$ + data[i + half] $\times Ig_1$ + data[i + 1] $\times Ig_2$ + data[i + halfplus] $\times Ig_3$
		\ENDFOR
		\ENDIF
	\end{algorithmic}
\end{algorithm}

\begin{algorithm}
	\caption{Principal Component Analysis Inference}
	\label{pca}
	\begin{algorithmic}[1]
		\REQUIRE
		Input: $\myvec{x} = (x_0, x_1, ..., x_{m-1})$, $\myvec{para}=(\myvec{U}, \myvec{x}_{center})$, where $\myvec{U}=(u_0,u_1,…,u_{k-1})$, $u_i$ is a $n$ dimensional vector, and $\myvec{x}_{center} = (x_{c0}, x_{c1}, ..., x_{c(m-1)})$
		\ENSURE
		The data after feature extraction: $\myvec{out}$ =  [$o_0, o_1, ..., o_{k-1}$]
		\FOR{$i = 0$; $i < k$; $i ++$}
		\STATE out[i] = $\myvec{u}_i$ $\cdot (\myvec{x}-\myvec{x}_{center})$ // calculate the inner product of $\myvec{u}_i$ and $(\myvec{x}-\myvec{x}_{center})$
		\ENDFOR
	\end{algorithmic}
\end{algorithm}

\begin{algorithm}
	\caption{Support Vector Machine Inference, (SVM)}
	\label{svm}
	\begin{algorithmic}[1]
		\REQUIRE
		Input: $\myvec{x} = (x_0, x_1, ..., x_{k-1})$. $\myvec{para}=(\myvec{x}_{sup}, \myvec{dc}, b)$, where $\myvec{x}_{sup}=(\myvec{x}_{sup0},\myvec{x}_{sup1},…,\myvec{x}_{sup(m-1)})$ is the support vectors, $\myvec{dc} = (\myvec{dc}_0, \myvec{dc}_{1}, ..., \myvec{dc}_{m-1})$ is the dual coefficients for each model, and $b$ is the intercept.
		\ENSURE
		The prediction result: $class$.
		\STATE temp = 0
		\FOR{$i = 0$; $i < m$; $i ++$}
		\STATE $s_i$ = 0
		\FOR{$j = 0$; $j < k$; $j++$}
		\STATE $s_i$ += $\mathsf{abs}(x_j - x_{supi}[j]) ^ 2$
		\ENDFOR
		\STATE $k_i = \mathsf{exp}(-\gamma \times s_j)$ //calculate the kernel function
		\STATE $temp$ += $c_i \times k_i$ 
		\ENDFOR
		\STATE decision = temp + b
		\IF{desicion$>0$}
		\STATE class = 1
		\ELSE
		\STATE class = 0
		\ENDIF
	\end{algorithmic}
\end{algorithm}

\thang{suggested structure}
\section{Introduction}

\section{Preliminaries}
\PP{Notation}

\PP{Argument of Knowledge}

\PP{Machine Learning (need to find more fancy words)}

\section{Models}
\PP{System Model}

\PP{Threat Model}

\PP{Security Model} \thang{Define zk verifiable machine learning definition}

\section{Proposed ZK and Verifiable Machine Learning Inference Framework}

\subsection{ML Inference Pipeline} 
\thang{Give a generic pipeline, starting from data input to classification output, 
	then categorize into two groups}

\PP{Data-Only Processing}

\PP{Model-Involved Data Processing}

\subsection{Gadgets and Functions}

\subsection{ZK ML Inference Instantiations}

\PP{Data Pre-processing / DWT}

\PP{Feature Extraction / PCA}

\PP{Inference / SVM}

\section{Security Analysis}

\thang{Prove the security of proposed technique according to the sec model definition in Models}

\section{Implementation}
\thang{describe detailed crypto primitive instantiations (commitments, hash etc.), zk-lib, crypto-lib used (take a look at Zcash paper to see how this part can be written nicely)} .
	
\section{Experimental Evaluation}

\subsection{System Setup, configuration and counterpart selection for comparison} 

\subsection{Overall Result}

\subsection{Detailed Cost}

\section{Conclusion}
